# Supplementary material for: Functional Frank-Wolfe Boosting for General Loss Functions
Source: arXiv:1510.02558 source file (2015-10-09)
Supplement: Supplementary file 1 [file supplement.pdf]

# Functional Frank-Wolfe Boosting for General Loss Functions: Supplementary Material

**Anonymous Author(s)**
Affiliation
Address
email

## Abstract

This note contains supplementary materials to *Functional Frank-Wolfe Boosting for General Loss Functions: Supplementary Material*.

## A Generalization error bounds on Functional Frank-Wolfe Boosting for General Loss Functions

### A.1 Proof of Theorem 3.2

Without loss of generality, we assume for any $h \in \mathcal{H}$, $-h \in \mathcal{H}$. In this way, all the $\alpha_t$ can be chosen to be non-negetive. We first show $\hat{\mathcal{R}}_S(\mathcal{F}_T^C) \leq C\hat{\mathcal{R}}_S(\mathcal{H}^1)$.

$$\begin{aligned}
& \hat{\mathcal{R}}_S(\mathcal{F}_T^C) \\
= \; & \mathbb{E}_\sigma[\sup_{f \in \mathcal{F}_T^C} \frac{1}{m} \sum_{i=1}^m \sigma_i f(x_i)] \\
= \; & \mathbb{E}_\sigma\Big[\sup_{h_t \in \mathcal{H}^D} \sup_{\alpha_t \in \mathbb{R}, \|\boldsymbol{\alpha}\|_1 \leq C} \frac{1}{m} \sum_{i=1}^m \sigma_i \sum_{t=1}^T \alpha_t h_t(x_i)\Big] \\
= \; & \mathbb{E}_\sigma\Big[\sup_{h_t \in \mathcal{H}^1} \sup_{\alpha_t \in \mathbb{R}, \|\boldsymbol{\alpha}\|_1 \leq C} \sum_{t=1}^T \alpha_t \big(\frac{1}{m} \sum_{i=1}^m \sigma_i h_t(x_i)\big)\Big] \\
\leq \; & \mathbb{E}_\sigma\Big[\sup_{h_t \in \mathcal{H}^1} \sup_{\alpha_t \in \mathbb{R}, \|\boldsymbol{\alpha}\|_1 \leq C} \sum_{t=1}^T \alpha_t \big(\sup_{h_t \in \mathcal{H}^1} \frac{1}{m} \sum_{i=1}^m \sigma_i h_t(x_i)\big)\Big] \\
= \; & \sup_{\alpha_t \in \mathbb{R}, \|\boldsymbol{\alpha}\|_1 \leq C} \sum_{t=1}^T \alpha_t \cdot \mathbb{E}_\sigma\Big[\sup_{h_t \in \mathcal{H}^1} \frac{1}{m} \sum_{i=1}^m \sigma_i h_t(x_i)\Big] \\
\leq \; & C\hat{\mathcal{R}}_S(\mathcal{H}^1).
\end{aligned}$$

Since for any function space $\mathcal{F}$ and $\mathcal{G}$, if $\mathcal{F} \subset \mathcal{G}$, $\hat{\mathcal{R}}_S(\mathcal{F}) \leq \hat{\mathcal{R}}_S(\mathcal{G})$, if base hypothesis space $\mathcal{H}$ is closed under scalar multiplication, then

$$C\hat{\mathcal{R}}_S(\mathcal{H}^1) \leq \hat{\mathcal{R}}_S(\mathcal{H}^C)$$

by the fact that $\forall h \in \mathcal{H}^1$, $C \cdot h \in \mathcal{H}^C$. By noting $\mathcal{H}^C \subset \mathcal{F}_T^C$, it is clear that $\hat{\mathcal{R}}_S(\mathcal{H}^C) \leq \hat{\mathcal{R}}_S(\mathcal{F}_T^C)$. Combining the above inequalities, we have $\hat{\mathcal{R}}_S(\mathcal{F}_T^C) \leq C\hat{\mathcal{R}}_S(\mathcal{H}^1) \leq \hat{\mathcal{R}}_S(\mathcal{H}^C) \leq \hat{\mathcal{R}}_S(\mathcal{F}_T^C)$, which completes the proof.

### A.2 Rademacher Complexity bounds for regression with $l_p$ loss

Combining this result with the general Rademahcer complexity learning bound of Theorem 3.1 yields the following Rademacher complexity bounds for regression with $l_p$ loss $l(a, y) = \frac{1}{p}|a - y|^p$.

**Theorem A.1.** *Suppose $y \in \mathcal{Y}$ is uniformly bounded by $A$ .Then for any $\delta > 0$, with probability at least $1 - \delta$ over a sample $S$ of size $m$, the following inequality holds for all $f \in \mathcal{F}^C$:*

$$\mathbb{E}\,[l_f] \leq \hat{\mathbb{E}}[l_f] + 2(A + C)^{p-1} C \hat{\mathcal{R}}_S(\mathcal{H}^1) + \frac{3}{p}(A + C)^p \sqrt{\frac{\log \frac{2}{\delta}}{2m}}.$$

*Proof.* For any $f \in \mathcal{F}_T^C$ and any $x \in \mathcal{X}, y \in \mathcal{Y}$, $|\sum_{t=1}^{T} \alpha_t h_t(x)| \leq \|\boldsymbol{\alpha}\|_1 \|h_t(x)\|_\infty \leq C$. Then from the assumption that $|y| \leq A$, we have $l_p$ loss is $(A + C)^{p-1}$-Lipschitz and $l(a, y) \leq \frac{1}{p}(A + C)^{p-1}$. We get the above inequality from Theorem 3.1 by setting $M = \frac{1}{p}(A + C)^{p-1}$ and incorporating Theorem 3.2. □

## B Bounds on Empirical Risk

### B.1 Proof of Theorem 3.3

By applying similar techniques in [1] to functional space and based on the definition of FW direction, we have

$$\langle h_t, \frac{\partial L}{\partial F_t} \rangle = \langle h_t, -\mathbf{r}_t \rangle = -\max_{s \in \mathcal{D}} \langle s, \mathbf{r}_t \rangle = \min_{s \in \mathcal{D}} \langle s, \frac{\partial L}{\partial F_t} \rangle.$$

Then we have

$$\langle h_t - F_t, \frac{\partial L}{\partial F_t} \rangle = \min_{s \in \mathcal{D}} \langle s, \nabla l \rangle - \langle F_t, \frac{\partial L}{\partial F_t} \rangle = \max_{s \in \mathcal{D}} \langle F_t - s, \frac{\partial L}{\partial F_t} \rangle.$$

Then we have

$$\begin{aligned} L(F_{t+1}, y) - L(F^*, y) &\leq L(F_t, y) - L(F^*, y) + \gamma_t \langle h - F_t, \frac{\partial L}{\partial F_t} \rangle + \frac{\gamma_t^2}{2} C_{l,\mathcal{F}} \\ &= L(F_t, y) - L(F^*, y) - \gamma_t \max_{s \in \mathcal{D}} \langle F_t - s, \frac{\partial L}{\partial F_t} \rangle + \frac{\gamma_t^2}{2} C_{l,\mathcal{F}} \\ &\leq L(F_t, y) - L(F^*, y) - \gamma_t \big( L(F_t, y) - L(F^*, y) \big) + \frac{\gamma_t^2}{2} C_{l,\mathcal{F}} \\ &= (1 - \gamma_t) \big( L(F_t, y) - L(F^*, y) \big) + \frac{\gamma_t^2}{2} C_{l,\mathcal{F}}, \end{aligned}$$

where the last inequality holds because of the convexity of $L$. For simplicity we use $p_t$ to denote $L(F_t, y) - L(F^*, y)$ and let $C^* = \max\{\frac{C_{l,\mathcal{F}}}{2}, \frac{3}{4} p_1\}$. Then immediately we have $p_1 \leq \frac{4C^*}{2+1}$. Now let $\gamma_t = \frac{2}{t+2}$, and assume we have $p_t \leq \frac{4C^*}{2+t}$, then by simple recursive relation, we have

$$p_{t+1} \leq (1 - \frac{2}{2+t}) \frac{4C^*}{2+t} + \frac{4}{(2+t)^2} C^* = \frac{4t+4}{(2+t)^2} C^* < \frac{4C^*}{2 + (t+1)}.$$

Notice that if we use line-search variant or fully-corrective variant at each iteration, the same bound holds. This is because $p_0^{LS}, p_0^{FC} = p_0$ and from $p_t^{LS}, p_t^{FC} \leq p_t$ it is straightforward to show that $p_{t+1}^{LS}, p_{t+1}^{FC} \leq p_{t+1}$. Then the same induction argument works, which completes the proof.

### B.2 Proof of Theorem 3.4

Following the same techniques in the proof of theorem 3.3, we have

$$\langle h_t - F_t, \frac{\partial L}{\partial F_t} \rangle \leq \min_{s \in \mathcal{D}} \langle s, \nabla l \rangle + \delta \gamma_t C_{l,\mathcal{F}} - \langle F_t, \frac{\partial L}{\partial F_t} \rangle = \max_{s \in \mathcal{D}} \langle F_t - s, \frac{\partial L}{\partial F_t} \rangle + \delta \gamma_t C_{l,\mathcal{F}}.$$

Then based on this we have

$$\begin{aligned} L(F_{t+1},y)-L(F^*,y) &\le L(F_t,y)-L(F^*,y)+\gamma_t\langle h-F_t,\frac{\partial L}{\partial F_t}\rangle+\frac{\gamma_t^2}{2}C_{l,\mathcal{F}} \\ &\le L(F_t,y)-L(F^*,y)-\gamma_t\max_{s\in\mathcal{D}}\langle F_t-s,\frac{\partial L}{\partial F_t}\rangle+\frac{\gamma_t^2}{2}(1+2\delta)C_{l,\mathcal{F}} \\ &\le L(F_t,y)-L(F^*,y)-\gamma_t\big(L(F_t,y)-L(F^*,y)\big)+\frac{\gamma_t^2}{2}(1+2\delta)C_{l,\mathcal{F}} \\ &= (1-\gamma_t)\big(L(F_t,y)-L(F^*,y)\big)+\frac{\gamma_t^2}{2}(1+2\delta)C_{l,\mathcal{F}}. \end{aligned}$$

Then by similar mathematical induction, we have

$$L(F_t,y)-L(F^*,y)\le\frac{C^*}{2+t}(1+2\delta).$$

### B.3 Stopping Criteria of FWBoost for $l_2$ Loss

**Proposition B.1.** *For $l_2$ loss, if the algorithm stops, it must stop at the global minimizer of the constrained optimization problem*

$$\begin{aligned} &\min_{\boldsymbol{\alpha}} L(\boldsymbol{\alpha})=\min_{\boldsymbol{\alpha}}\frac{1}{2}\sum_{i=1}^{m}\Big[y_i-\sum_j a_j h_j(x_i)\Big]^2 \\ &\text{s.t. } \ ||\boldsymbol{\alpha}||_1\le C,\ \ a_j\ge 0,\ j=1,2,\cdots,|\mathcal{H}|. \end{aligned}$$

*Proof.* Suppose at time $t$ the algorithm stops at $\boldsymbol{\alpha}^*=(\alpha_1,\alpha_2,\ldots,\alpha_{|\mathcal{H}|})$ be the stopped position. First of all, notice that the initial position of the algorithm is feasible and $\boldsymbol{\alpha}$ will remain in the feasible domain during the adjustment of the weights. Therefore the stopped position $\boldsymbol{\alpha}^*$ is also feasible.

Since the objective function is convex, the inequality constraints are continuously differentiable convex functions and the equality constraints are affine functions, we only need to show that $\boldsymbol{\alpha}^*$ satisfies Karush-Kuhn-Tucker conditions.

The algorithm stops as $\boldsymbol{\alpha}^*$. Then it follows that $s_t-F_{t-1}$ is not a descend direction. Suppose that the weak learner fitted at time $t$ is $h_k$. The gradient of the objective function is computed explicitly as

$$\nabla L(\boldsymbol{\alpha})=-(\langle\mathbf{r},h_1\rangle,\langle\mathbf{r},h_2\rangle,\ldots,\langle\mathbf{r},h_n\rangle).$$

Then the fact that $s_t-F_{t-1}$ is not a descend direction means

$$\langle\mathbf{r},h_k\rangle\le\sum_j\alpha_j\langle\mathbf{r},h_j\rangle.$$

However, $h_k$ is obtained by fitting the residue $\mathbf{r}$, then it follows that

$$h_k=\arg\max_{1\le i\le|\mathcal{H}|}\langle\mathbf{r},h_i\rangle.$$

Then we have

$$\langle\mathbf{r},h_k\rangle\le\sum_j\alpha_j\langle\mathbf{r},h_j\rangle\le\langle\mathbf{r},h_k\rangle\sum_j\alpha_j\le\langle\mathbf{r},h_k\rangle.$$

If $\boldsymbol{\alpha}^*$ is an interior point of the feasible region $|\boldsymbol{\alpha}|_1\le 1$, then the last inequality implies that $\mathbf{r}\cdot h_i=0$ for all $1\le i\le\mathcal{H}$, which means $\nabla L(\boldsymbol{\alpha})=0$.

On the other hand, if $\boldsymbol{\alpha}^*$ is on the boundary of the feasible region, then the last inequality implies that $\mathbf{r}\cdot h_i=\mathbf{r}\cdot h_k$ for all $1\le i\le\mathcal{H}$, which means the gradient $\nabla L(\boldsymbol{\alpha})$ is in the same direction of the outer normal of the feasible region $|\boldsymbol{\alpha}|_1\le 1$. This ensures that $\boldsymbol{\alpha}^*$ satisfies the KKT conditions. □

## C Frank-Wolfe boosting with away steps

A variant of the Frank-Wolfe algorithm, the so-called away step method, aims to solve the optimization problem while keeping the variable sparse. Since in real applications, especially in web applications, shorter querying time is essential for user experience. Predictors that use only a small subset of base hypotheses require a smaller memory footprint and can be applied faster. Thus keeping the parameter vector $\boldsymbol{\alpha}$ sparse during the iteration is desirable.

Guélat and Marcotte [2] developed the algorithm with away steps to directly solve the sparsity problem . Here we provide the away-step variant of Frank-Wolfe boosting method (in Algorithm 1), which directly solves the $l_1$ constrained regression problem while maintaining the sparsity of the base hypothesis by away-steps that potentially remove an old base hypothesis with bad performance.

**Algorithm 1:** Frank-Wolfe Gradient Boosting with awaystep

**input** : $m$ examples $(x_1, y_1) \dots (x_m, y_m)$ and constant $C$
Set $\mathcal{I}_1 = \emptyset$

**for** $t = 1, 2, 3, \dots T$ **do**
    $r_{t,i} = -\left[\frac{\partial L(y_i, F(x_i))}{\partial F(x_i)}\right]_{F(x)=F_{t-1}(x)}, \quad i = 1, \dots, m$
    Solve the subproblem $h_t = C \cdot \arg\min_{h \in \mathcal{H}^1} \langle h, \boldsymbol{r}_t \rangle$, define FW direction $d_t = h_t - F_{t-1}$
    Solve the subproblem $h_{min} = \arg\min_{h \in \mathcal{I}_t} \langle h, \boldsymbol{r}_t \rangle$, define away direction $d_t^A = F_{t-1} - Ch_{min}$
    **if** $d_t^{FW} \cdot \boldsymbol{r}_t > d_t^A \cdot \boldsymbol{r}_t \mid\mid t == 1$ **then**
        $\gamma_t^{FW} = \arg\min_{\gamma \in [0,1]} \sum_{i=1}^m L\big(y_i, F_{t-1}(x_i) + \gamma d_t^{FW}(x_i)\big)$
        Perform the FW step $\alpha_k \leftarrow (1 - \gamma_t^{FW})\alpha_k$ for $h_k \in \mathcal{I}_t$ and $\alpha_t^{FW} = \gamma_t^{FW} C$
        Let $h_t^{FW} = h_t / C$ and update $\mathcal{I}_t$ by $\mathcal{I}_{t+1} = \mathcal{I}_t \cup \{h_t^{FW}\}$
        $F_t = F_{t-1} + \gamma_t^{FW} d_t^{FW}$
    **else**
        $\gamma_t^A = \big\{\alpha_{min}/(C - \alpha_{min}), \arg\min_{\gamma \in [0,1]} \sum_{i=1}^m L\big(y_i, F_{t-1}(x_i) + \gamma d_t^A(x_i)\big)\big\}$
        Perform the away step $\alpha_k \leftarrow (1 + \gamma_t^A)\alpha_k$ for $h_k \neq h_{min}$ and
        $\alpha_t^{FW} = (1 + \gamma_t^{FW})\alpha_t^{FW} - \gamma_t^{FW} C$
        **if** $\gamma_t^A = \alpha_{min}/(C - \alpha_{min})$ **then** $\mathcal{I}_{t+1} = \mathcal{I}_t \backslash \{h_{min}\}$
        $F_t = F_{t-1} + \gamma_t^A d_t^A$
    **end**
**end**
**output**: $F_T(x)$

## References


[1] Martin Jaggi. Revisiting frank-wolfe: Projection-free sparse convex optimization. In *Proceedings of the 30th International Conference on Machine Learning (ICML-13)*, pages 427–435, 2013.

[2] Jacques Guélat and Patrice Marcotte. Some comments on wolfe's away step. *Mathematical Programming*, 35(1):110–119, 1986.
